# Supplementary material for: Coherent control at its most fundamental: CEP-dependent electron localization in photodissoziation of a H2+ molecular ion beam target
Source: arXiv:1306.1755 ancillary file (2013-09-20)
Supplement: Supplementary file 1 [file Supp_Mat.pdf]

## I. EXPERIMENTAL SETUP

Few-cycle (4.5 fs = 1.5 cycles) 400-$\mu$J laser pulses are produced at a repetition rate of 4 kHz in a hollow-core fiber compressor (central wavelength 750 nm), driven by a 1-mJ Ti:sapphire laser system (Femtopower Compact Pro by Femtolasers). The beam is divided by an ultra-broadband beam splitter such that 30% are focused into the phasemeter and 70% into the ion beam apparatus perpendicularly to the ion beam. Intensities up to $(4 \pm 2) \times 10^{14}\,\mathrm{W/cm^2}$ are obtained, see also Fig. 1. The spectral dispersion in both paths is compensated with fused silica wedges to achive the shortest possible pulse.

The ion beam ($E_{kin}$=8 keV) is generated in a duoplasmatron ion source similarly to [1]. For mass and charge separation a Wien filter is used. Deflector plates, Einzel lenses, and adjustable slits control and collimate the beam down to a diameter of less than 200 $\mu$m. The electric field generated by the ion spectrometer induces a time delay between the charged and neutral fragments thus allowing for a clear distinction between the two fragments. A time- and position-sensitive delay-line detector is used to record the fragments in coincidence. The total length of the ion beam setup is 7 m and the pressure inside the apparatus $7 \times 10^{-9}$ mbar. The stereo-ATI phasemeter measures the absolute phase $\phi$ of each laser pulse (single shot error <100 mrad) [2, 3]. In this way, a phase-resolved and kinematically complete measurement is realized from which the phase dependence of the kinetic energy release (KER)-spectra and electron localization can be determined. This phase-tagging setup allows long term (tens of hours) and high precision absolute-phase sensitive measurements.

To highlight the asymmetry between 0.5 and 1.4 eV, the data from Fig. 3a is replotted in Fig. S.1. The false color scale has been modified and contour lines for zero asymmetry have been added to guide the eye. Here we see that the CEP-dependence of the asymmetry rapidly changes by $\sim 360°$ in the region between 0.25 and 0.75 eV and has a magnitude of $\sim 3\%$.

## II. THEORETICAL METHOD

The time-dependent Schrödinger equation (TDSE) calculation, including nuclear rotation [4, 5], employed here will be briefly summarized for completeness. The full Hamiltonian is (in atomic units)

$$H = -\frac{1}{2\mu}\nabla_R^2 + H_{\mathrm{el}} - \boldsymbol{\mathcal{E}}(t) \cdot \mathbf{d} \tag{1}$$

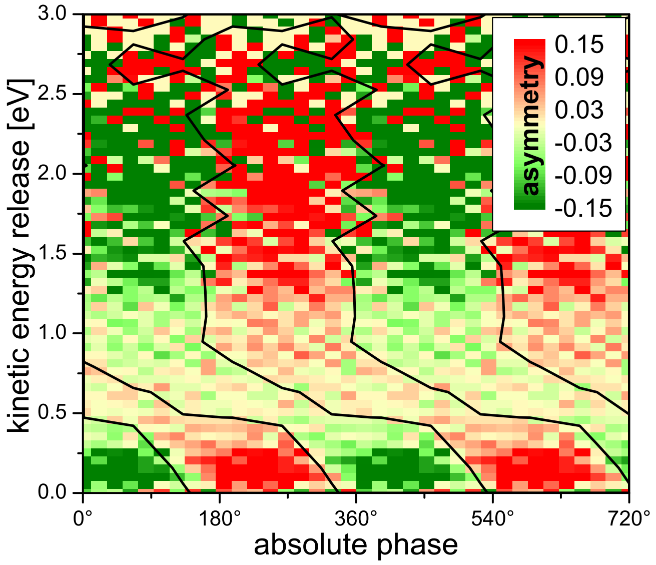


FIG. S.1. Alternative view of the measured asymmetry of the bound electron with a few-cycle laser pulse (4.5 fs). The data is taken from Fig. 3a and the false color scale is modified to highlight the asymmetry for the energy region between 0.5 and 1.4 eV. The contour lines mark zero asymmetry to guide the eye.

where $H_{\rm el}$ is the electronic Hamiltonian, $R$ designates the nuclear degrees of freedom, and $\mu$ is the nuclear reduced mass. We use the length gauge with $\boldsymbol{\mathcal{E}}(t)$ the instantaneous electric field and $\mathbf{d}$ the dipole operator. The electric field is obtained from the Fourier transform of the pulse's measured power spectrum $I(\omega)$:

$$\mathcal{E}(t) = \int_{-\infty}^{\infty} \sqrt{I(\omega)} e^{-i[\omega t + \varphi(\omega)]}\, d\omega \tag{2}$$

where $I(-\omega) = I(\omega)$ and $\varphi(-\omega) = -\varphi(\omega)$ ensure that the instantaneous field is real. We have assumed that the spectral phase is flat, corresponding to the transform limit of the measured spectrum, in which case $\varphi(\omega) = \varphi$ (when $\omega > 0$) defines the carrier-envelope phase (CEP). This transform-limited pulse is illustrated in Fig. S.2.

We expand the total wave function on the electronic states $\Phi_\beta$ and on the angular momentum function $\Omega^{J\pi}_{\Lambda M}$ defined in terms of Wigner $D$-functions to represent the nuclear rotation [4],

$$\Psi(\mathbf{R}, \mathbf{r}, t) = \sum_\alpha F_\alpha(R, t)\Omega^{J\pi}_{\Lambda M}(\theta, \phi)\Phi_\beta(R; \mathbf{r}), \tag{3}$$

where $\theta$ and $\phi$ are the nuclear spherical polar angles (the nuclear axis points from proton $A$ to proton $B$) and $\mathbf{r}$ is the molecular-frame electronic coordinate. The index $\beta$ represents the quantum

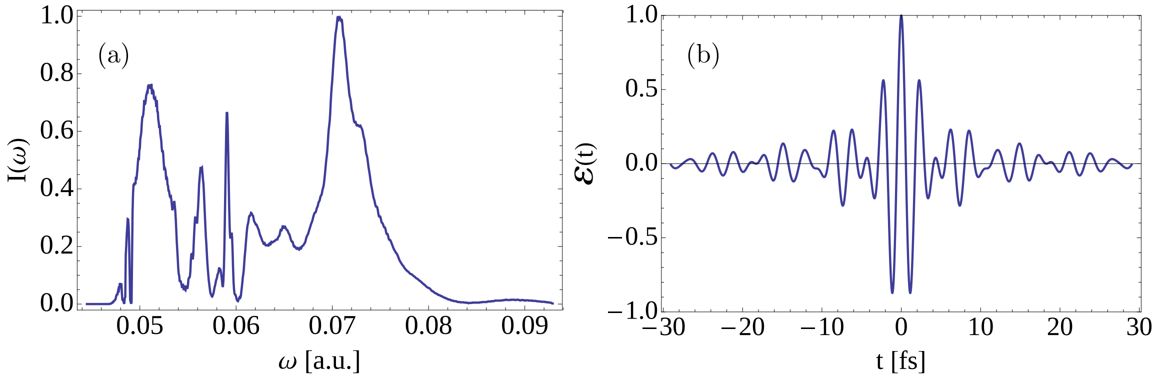


FIG. S.2. (a) The measured power spectrum of the pulse. (b) The time-dependent field retrieved from the Fourier transform of the power spectrum with $\varphi = 0$.

numbers needed to specify the electronic state, and $\alpha$ collectively denotes all quantum numbers — i.e., $\alpha \equiv (\beta J M \pi)$. In this basis, the TDSE becomes

$$i\frac{\partial}{\partial t}F_\alpha = \left(-\frac{1}{2\mu}\frac{\partial^2}{\partial R^2} + \frac{J(J+1)-\Lambda^2}{2\mu R^2} + U_\beta(R)\right)F_\alpha - \boldsymbol{\mathcal{E}}(t)\cdot\sum_{\alpha'}\langle\Phi_\beta\Omega^{J\pi}_{\Lambda M}|\mathbf{d}|\Phi_{\beta'}\Omega^{J'\pi'}_{\Lambda' M'}\rangle F_{\alpha'} \quad (4)$$

where $U_\beta(R)$ is the Born-Oppenheimer potential.

Through numerical testing, we have confirmed that the $n = 2$ excited manifold of electronic channels plays a negligible role in determining the asymmetry for a Gaussian pulse with roughly the same parameters as the measured pulse. In fact, ensuring that this result held — and thus presumably that ionization was also negligible — led to the limited intensity used in the theory. Consequently, the calculations presented included only the $1s\sigma_g$ and $2p\sigma_u$ channels. Taken together with the initial condition that $J = 0$, $\alpha$ can be simplified to $\beta, J$ which will be the preferred label in the remainder of this note. In principle, an initially thermal distribution of ro-vibrational states should be used rather than $J = 0$. We have found [5], however, that the relative momentum distribution of $p + \mathrm{H}$ fragments upon performing the sum over all $M$s for a given $J$ are nearly indistinguishable from that of $J = 0$. We thus present only $J = 0$ results which also reduces the computational resources required by one to two orders of magnitude.

Given our restriction to just $1s\sigma_g$ and $2p\sigma_u$ channels, Eq. (4) is exact. We propagate the wave functions in time using a split operator scheme combined with Crank-Nicolson. Since the narrow peaks in the power spectrum give rise to long tails for the pulse in the time domain, we had to extend the propagation to over 700 fs in total with a time step of 1.0 a.u. and a box of 400 a.u. to achieve convergence to 3 digits in the total dissociation probability for a given vibrational state.

We further ensured this convergence held with respect to all other numerical parameters. Under these conditions, the resulting asymmetry $\mathcal{A}$ is converged to within 1% of the maximum asymmetry amplitude. These statements apply within the restriction of the electronic basis to $1s\sigma_g$ and $2p\sigma_u$. When the basis is expanded to include the $n = 2$ manifold, we estimate that the error in $\mathcal{A}$ might grow to 5–10% based on some numerical tests for similar laser parameters. Each initial vibrational state ($v$=0–19 for $H_2^+$) is propagated independently and its physical observables computed. These individual observables are then summed together, weighted by the Franck-Condon factors, to obtain the final observables.

To make the comparison between theory and experiment as quantitative as possible, we average the final observables over the intensity distribution within the reaction volume based on the geometry of the experimental setup [6]. We assume that the transverse intensity profile of the laser beam is Gaussian, $I(r) = I_0 e^{-(\frac{r}{\Delta r})^2}$ characterized by its width $\Delta r$. Then, the intensity average of some observable $P$ for peak intensity $I_0$ can be evaluated from

$$\begin{aligned} \bar{P}(I_0) &\propto \int_0^\infty P[I(r)] 2\pi r dr \\ &= \int_0^{I_0} P(I) \frac{dI}{I} \ . \end{aligned} \quad (5)$$

This procedure thus emphasizes the contributions from the volumes where the intensity is lower than $I_0$. The intensity-averaging step is clearly crucial for comparing theory and experiment quantitatively, but it also makes a *qualitative* change in calculated observables.

## III. PATHWAYS FOR COHERENT CONTROL

It has been established [7, 8] that a particularly convenient and powerful way to think about CEP effects is that they result from the interference of different photon pathways. For instance, CEP-dependent spatial asymmetry is a consequence primarily of the interference of $n$ and $n + 1$ photon pathways since they produce final states of opposite parity — the necessary condition for breaking spatial symmetry. As discussed in the main text, this interference can only occur between indistinguishable pathways connecting the same initial and final states. For $H_2^+$, the pathways must begin with the same vibrational state and end at the same KER. Thus, KER regions in which the contributions from the $|1s\sigma_g - n\omega\rangle$ and $|2p\sigma_u - (n \pm 1)\omega\rangle$ final states are roughly equal will have the greatest possibility to create an asymmetry since dipole selection rules dictate that these pathways will populate nuclear angular momentum states with opposite parity.

Figure S.3 shows, for instance, the $1s\sigma_g$ and $2p\sigma_u$ KER spectra separately for an initial $v = 6$

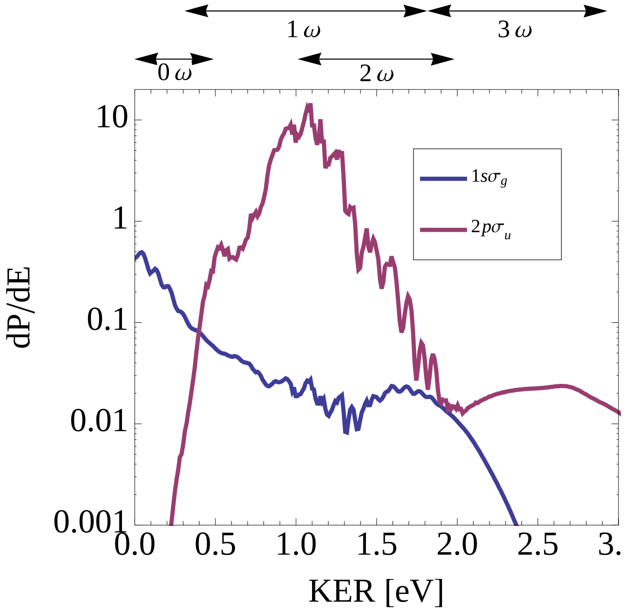


FIG. S.3. The intensity-averaged and CEP-averaged $1s\sigma_g$ and $2p\sigma_u$ KER distributions at $I_0 = 1.0 \times 10^{14}$ W/cm$^2$ for the $v = 6$ vibrational level. Note that, as expected, the KER regions where the probabilities for dissociation along $1s\sigma_g$ and $2p\sigma_u$ are roughly equal are the regions where the largest asymmetries appear in Fig. 3. The rough KER ranges for $n$-photon dissociation are marked along the top of the figure.

state. The indicated net photon numbers are marked approximately based on the KER. From this figure, one would thus expect CEP effects near 0.4 eV and 1.9 eV. Of course, the contributions from different initial vibrational states can have different CEP dependence at those KER, which will tend to wash out the effect. Therefore, both a roughly equal contribution from different pathways and similar CEP dependence from different vibrational states are required to produce a large asymmetry in the experimental observable.

Since the experimental observable is an incoherent sum over the initial states, it is instructive to examine the contribution from individual initial states. To this end, Fig. S.4 shows the total dissociation probability for each initial vibrational state. The figure also shows the total weight of each vibrational state in the observable total dissociation probability. Figure S.4(b) shows that the $v = 8$–$12$ states contribute the most to the total yield, and they do so through the net one-photon bond-softening process. These states can also dissociate with zero net photons, leading to CEP-dependent interference at low KER. The $v < 7$ states are primarily responsible for the asymmetry at high KER. Although the lower vibrational states are relatively far away from the one-photon crossing, they are reasonably close to the three-photon crossing. These states can absorb one net

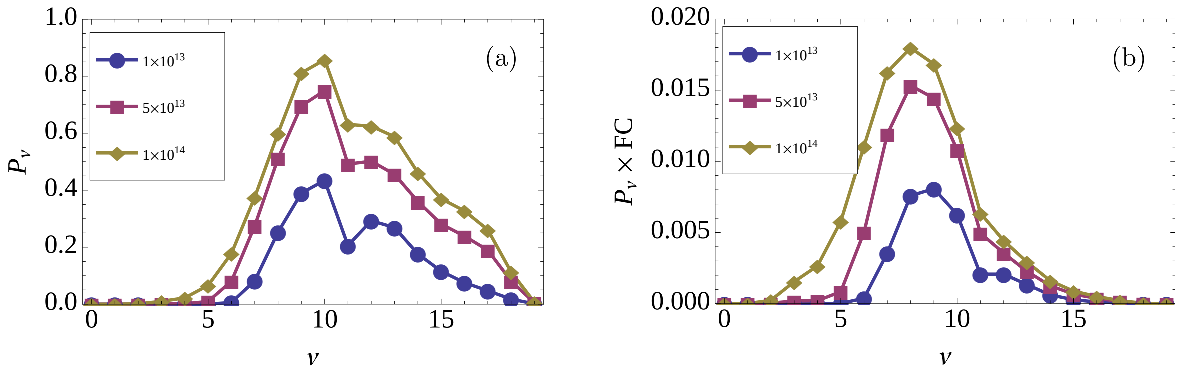


FIG. S.4. (a) The total dissociation probability $P$ as a function of vibrational state for various peak intensities. (b) The total weight for each initial state, which is the Franck-Condon factor times the total dissociation probability.

photon to dissociate directly or they can absorb three photons and emit one for a net two-photon dissociation. The lower probability of a three-photon transition compared to one photon is thus compensated by the states' being closer to the three-photon crossing (see Fig. 2a). As we increase the peak intensity, the contribution from these lower vibrational states becomes more important as Fig. S.4(b) shows. It is likely that they will grow even further beyond $10^{14}$ W/cm$^2$ and produce larger asymmetries, possibly explaining the discrepancy in the asymmetry's magnitude between theory and experiment.

## IV. ELECTRONIC DYNAMICS

To visualize the electronic dynamics within the molecule, we can calculate the electron density $\rho(\mathbf{r},t)$ from the total wave function, Eq. (3), as

$$\begin{aligned}\rho(\mathbf{r},t) &= \int d^3R\,|\Psi(\mathbf{R},\mathbf{r},t)|^2 \\ &= \int d^3R\left|\sum_{\beta,J} F_{\beta J}(R,t)Y_{J0}(\theta,\phi)\Phi_\beta(R;\mathbf{r})\right|^2. \end{aligned} \tag{6}$$

Note that with the restriction to only $\beta$=$1s\sigma_g$ and $2p\sigma_u$ and with $J=0$ initially, $\Omega^{J\pi}_{\Lambda M}$ reduces to a spherical harmonic. Expanding the square and evaluating the integral gives

$$\rho(\mathbf{r},t) = \sum_{\beta,J}\int dR\,|F_{\beta J}(R,t)|^2|\Phi_\beta(R;\mathbf{r})|^2. \tag{7}$$

Recalling that $\mathbf{r}$ is the molecular-frame electronic coordinate, the asymmetry we seek should appear as a function of $\tilde{z}$ where the tilde indicates a molecular-frame coordinate. Given that $|\Phi_{1s\sigma_g}|^2$ and $|\Phi_{2p\sigma_u}|^2$ are even under $\tilde{z} \to -\tilde{z}$, we see that $\rho(\mathbf{r}, t)$ displays no asymmetry.

To observe any asymmetry in the electronic density, then, we must also consider the nuclear degrees of freedom. In particular, the integral in Eq. (6) must be restricted to a range of $\theta$ asymmetric about $\theta{=}\pi/2$. A natural choice is to integrate over the range $0 \leq \theta \leq \frac{\pi}{2}$, corresponding physically to proton $B$ lying in the upper hemisphere in the laboratory frame whether it is bound or free. The electron may or may not be bound to this proton, so such a quantity does not correspond to the physically observable $p$+H momentum distribution in which an H leaves into the upper hemisphere and a $p$ leaves into the lower hemisphere. Explicitly, the electron density as a function of the molecular-frame $\tilde{z}$ coordinate given that proton $B$ lies in the upper hemisphere in the laboratory frame is ($g \equiv 1s\sigma_g$ and $u \equiv 2p\sigma_u$)

$$\rho(\tilde{z}, t) = \frac{1}{2}\int_0^\infty dR \int d\tilde{x} d\tilde{y} \left[ \sum_{J \text{ even}} |F_{gJ}(R,t)|^2 \, |\Phi_g(R;\mathbf{r})|^2 + \sum_{J \text{ odd}} |F_{uJ}(R,t)|^2 \, |\Phi_u(R;\mathbf{r})|^2 \right] + \frac{1}{2}\,\mathrm{Re} \int_0^\infty dR \int d\tilde{x} d\tilde{y}\, \Phi_g(R;\mathbf{r}) \Phi_u(R;\mathbf{r}) \sum_{\substack{J' \text{ even} \\ J \text{ odd}}} f_{J'J} F^*_{gJ'}(R,t) F_{uJ}(R,t) \quad (8)$$

where

$$f_{J'J} = \frac{(-1)^{(J'+J+1)/2} J! J'! \sqrt{2J'+1}\sqrt{2J+1}}{2^{J'+J-1}(J'-J)(J'+J+1)\left[(\frac{1}{2}J')!\right]^2 \left\{\left[\frac{1}{2}(J-1)\right]!\right\}^2}. \quad (9)$$

It is this scenario that is shown in Fig. 5.


[1] H. Liebl and W.W. Harrison, Int. J. Mass Spectrom. Ion Phys. **22,** 237–246 (1976).

[2] T. Rathje *et al.*, J. Phys. B: At. Mol. Opt. Phys. **45,** 074003 (2012).

[3] T. Wittmann *et al.*, Nat. Phys. **5,** 357–362 (2009).

[4] F. Anis and B. D. Esry. *Phys. Rev. A* **77,** 33416 (2008).

[5] F. Anis, *Ph.D. thesis*, Kansas State University (2009).

[6] S. Zeng and B. D. Esry, to be published

[7] V. Roudnev and B. D. Esry, *Phys. Rev. Lett.* **99,** 220406 (2007).

[8] J. J. Hua and B. D. Esry, *J. Phys. B: At. Mol. Opt. Phys.* **42,** 85601 (2009).
